# Supplementary material for: Scalable Bayesian Uncertainty Quantification for Neural Network Potentials: Promise and Pitfalls
Source: arXiv:2212.07959 ancillary file (2023-07-27)
Supplement: Supplementary file 1 [file Supplement.pdf]

# Scalable Bayesian Uncertainty Quantification for Neural Network Potentials: Promise and Pitfalls - Supporting Information

Stephan Thaler[1], Gregor Doehner[1], and Julija Zavadlav[1,2]

[1] *Professorship of Multiscale Modeling of Fluid Materials, Department of Engineering Physics and Computation, TUM School of Engineering and Design, Technical University of Munich, Germany*
[2] *Munich Data Science Institute, Technical University of Munich, Germany*

## Contents

**Supplementary Methods** **1**
1. Prior Potential . . . . . . . . . 1
2. Lennard Jones Training . . . . . . . . . 1
3. Pressure Matching . . . . . . . . . 2

**Supplementary Figures** **3**

**Supplementary References** **11**

# Supplementary Methods

## 1. Prior Potential

In the common case of generating a data set by sampling from the Boltzmann distribution defined by the underlying high-fidelity model, e.g. via a molecular dynamics (MD) simulation, the resulting data set contains mostly states near energy minima, few high-energy states and no unphysical states such as overlapping atoms. Due to their data-driven nature, NN potentials are unconstrained in phase-space regions not contained in the training data set. When using such a NN potential in MD simulations, the simulation state may reach these unconstrained phase-space regions, resulting in unphysical or highly inaccurate potential energy predictions [1, 2] that often result in numerical instability [3]. This is exacerbated for CG potentials, which are designed to reach time and length scales inaccessible to the data-generating AT model.

Classical potentials avoid this problem by using physics-inspired functional forms [4, 5] that encode a priori known physical principles. For example, the Lennard Jones potential encodes repulsion due to the Pauli exclusion principle at close distances and Van-der-Walls attraction at larger distances. Eq. (11) in the main text casts training the NN potential as $\Delta$-learning [6], where the NN potential corrects an a priori chosen classical potential in phase-space regions where training data are available. With this ansatz, the goal of the prior potential is to enforce qualitatively correct predictions where the NN potential is unconstrained, especially for (unphysical) high-energy states, in order to drive the MD simulation back into the training data distribution, where the NN potential is accurate [7].

For the considered examples with the DimeNet++ [8, 9] potential, the prior potential increases simulation stability significantly compared to the case without it [3]. We found that the specific parameters of the prior potential typically have a minor effect on simulation results [10, 7], assuming the chosen prior successfully restricted the MD simulation from entering unphysical phase-space regions.

## 2. Lennard Jones Training

We generate 7500 samples using the No-U-Turn Sampler (NUTS) [11], of which 4100 are discarded during warm-up. For the Deep Ensemble [12, 13] and the preconditioned Stochastic Gradient Langevin Dynamics (pSGLD) methods, we employ a batch size of 1 as well as an initial learning rate of 0.01 and a final learning rate of $5 \cdot 10^{-5}$, with all

intermediate learning rates being set via a polynomial step size schedule [14]. We train models of the former for 10000 epochs and run chains for 10000 epochs for the latter, where 8000 were discarded as burn-in.

## 3. Pressure Matching

The pressure $P$ can be computed from the following relation [15]:

$$P = \frac{N_{\mathrm{DOF}} k_{\mathrm{B}} T}{3V} + \frac{\langle W \rangle}{3V} \ , \tag{1}$$

with temperature $T$, Boltzmann constant $k_{\mathrm{B}}$, volume $V$, ensemble averaged internal virial $\langle W \rangle$ and number of degrees of freedom in the system $N_{\mathrm{DOF}}$. We augment the FM loss with a virial-matching term [16], which we weight by $w_{\mathrm{P}} = 0.1$

$$L(\boldsymbol{\theta}) = \frac{1}{N_{\mathrm{F}}} \sum_{j=1}^{N_{\mathrm{F}}} [F_j - F_{j,\boldsymbol{\theta}}]^2 + \frac{w_{\mathrm{p}}}{N_{\mathrm{box}}} \sum_{k=1}^{N_{\mathrm{box}}} \left[ \frac{W_k^i}{3V} - \frac{W_{k,\boldsymbol{\theta}}}{3V} \right]^2 \ , \tag{2}$$

where $W_k^i/(3V)$ is the target instantaneous internal virial term, $W_{k,\boldsymbol{\theta}}/(3V)$ is the internal virial term of state $k$ predicted by the NN potential with parameters $\boldsymbol{\theta}$ and the definition of the first term is given in eq. (9) in the main text.

Similar to approaches in the literature [17], we employ an iterative pressure matching scheme. We adjust the internal virial values of the atomistic (AT) trajectory $W_k^{\mathrm{AT}}$ to account for the smaller kinetic energy of the CG system to obtain the initial targets:

$$\frac{W_k^0}{3V} = \frac{W_k^{\mathrm{AT}}}{3V} + \frac{k_{\mathrm{B}} T}{3V} (N_{\mathrm{DOF}}^{\mathrm{AT}} - N_{\mathrm{DOF}}^{\mathrm{CG}}) \ . \tag{3}$$

The iterative scheme then accounts for differences in the pressure due to the distribution shift between the mapped AT trajectory and the trajectory sampled by the CG model:

$$\frac{W_k^{i+1}}{3V} = \frac{W_k^i}{3V} + P^{\mathrm{AT}} - P_{\boldsymbol{\theta}}^{i,\mathrm{CG}} \ , \tag{4}$$

where $P^{\mathrm{AT}}$ is the AT reference pressure and $P_{\boldsymbol{\theta}}^{i,\mathrm{CG}}$ is the pressure obtained from a CG MD simulation with model parameters $\boldsymbol{\theta}$ at iteration $i$. We obtained acceptable models after the third iteration.

# Supplementary Figures

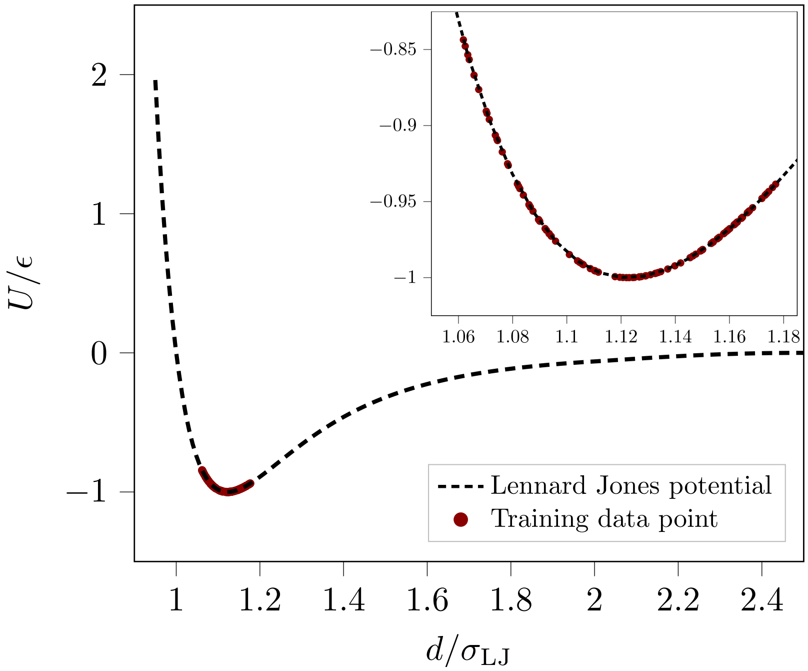


Figure 1: Lennard Jones potential. Data-generating Lennard Jones potential with sampled training data points and zoom on the training interval.

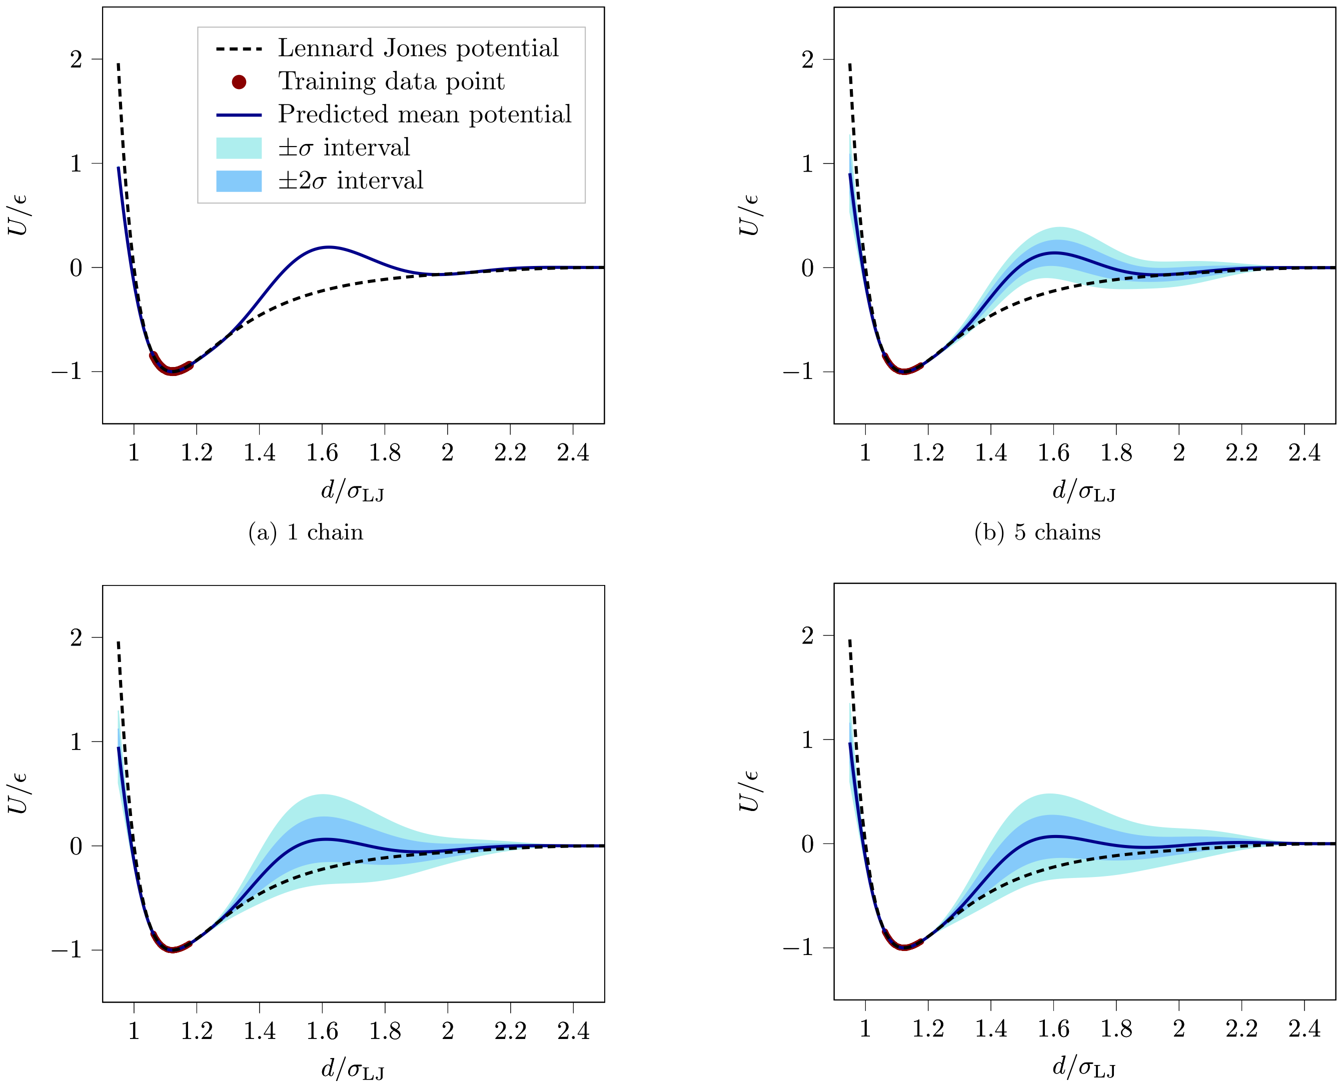


(a) 1 chain

(b) 5 chains

(c) 8 chains

(d) 10 chains

Figure 2: Chain convergence of the No-U-Turn Sampler. Predicted mean potential with $\pm\sigma$ and $\pm 2\sigma$ intervals of the No-U-Turn Sampler (NUTS) with samples collected from 1 ($a$), 5 ($b$), 8 ($c$) and 10 chains ($d$) – compared to the Lennard Jones reference.

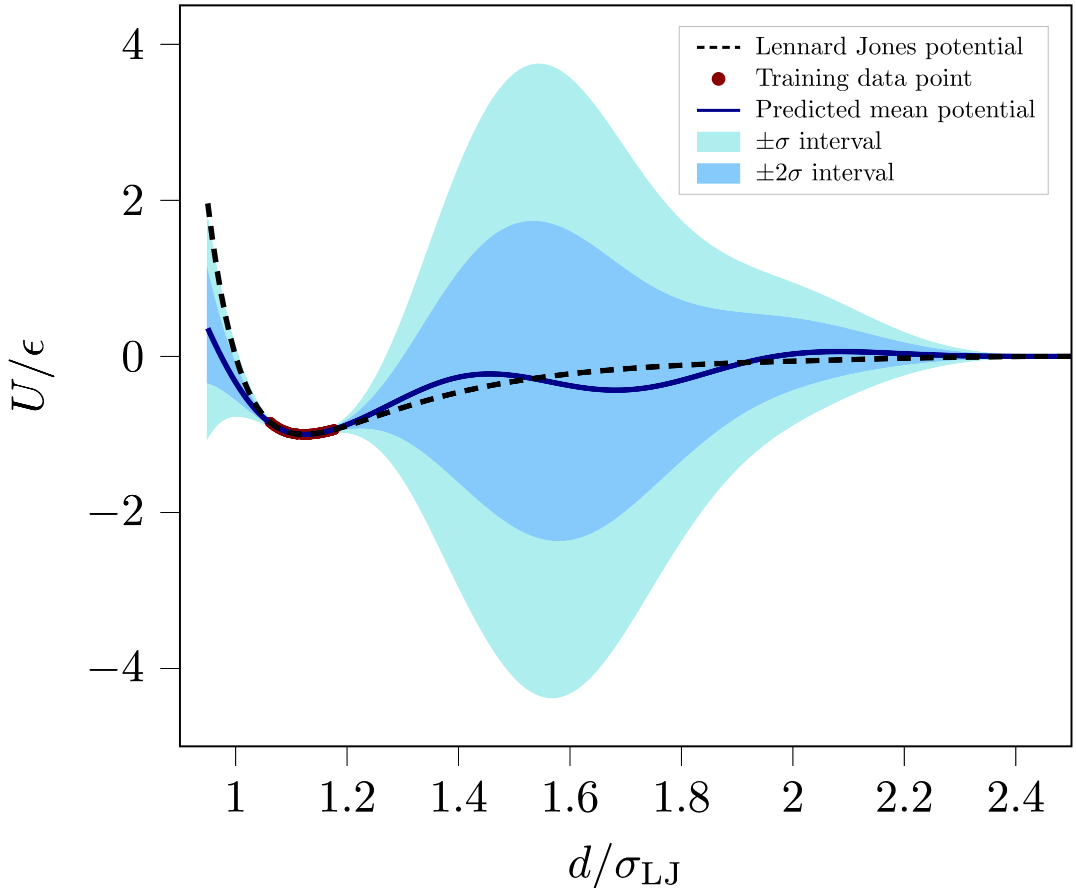


Figure 3: Single chain No-U-Turn Sampler (NUTS) with fixed $\sigma_{\mathrm{H}} = 0.05$. Predicted mean potential with $\pm\sigma$ and $\pm 2\sigma$ intervals compared to the Lennard Jones reference.

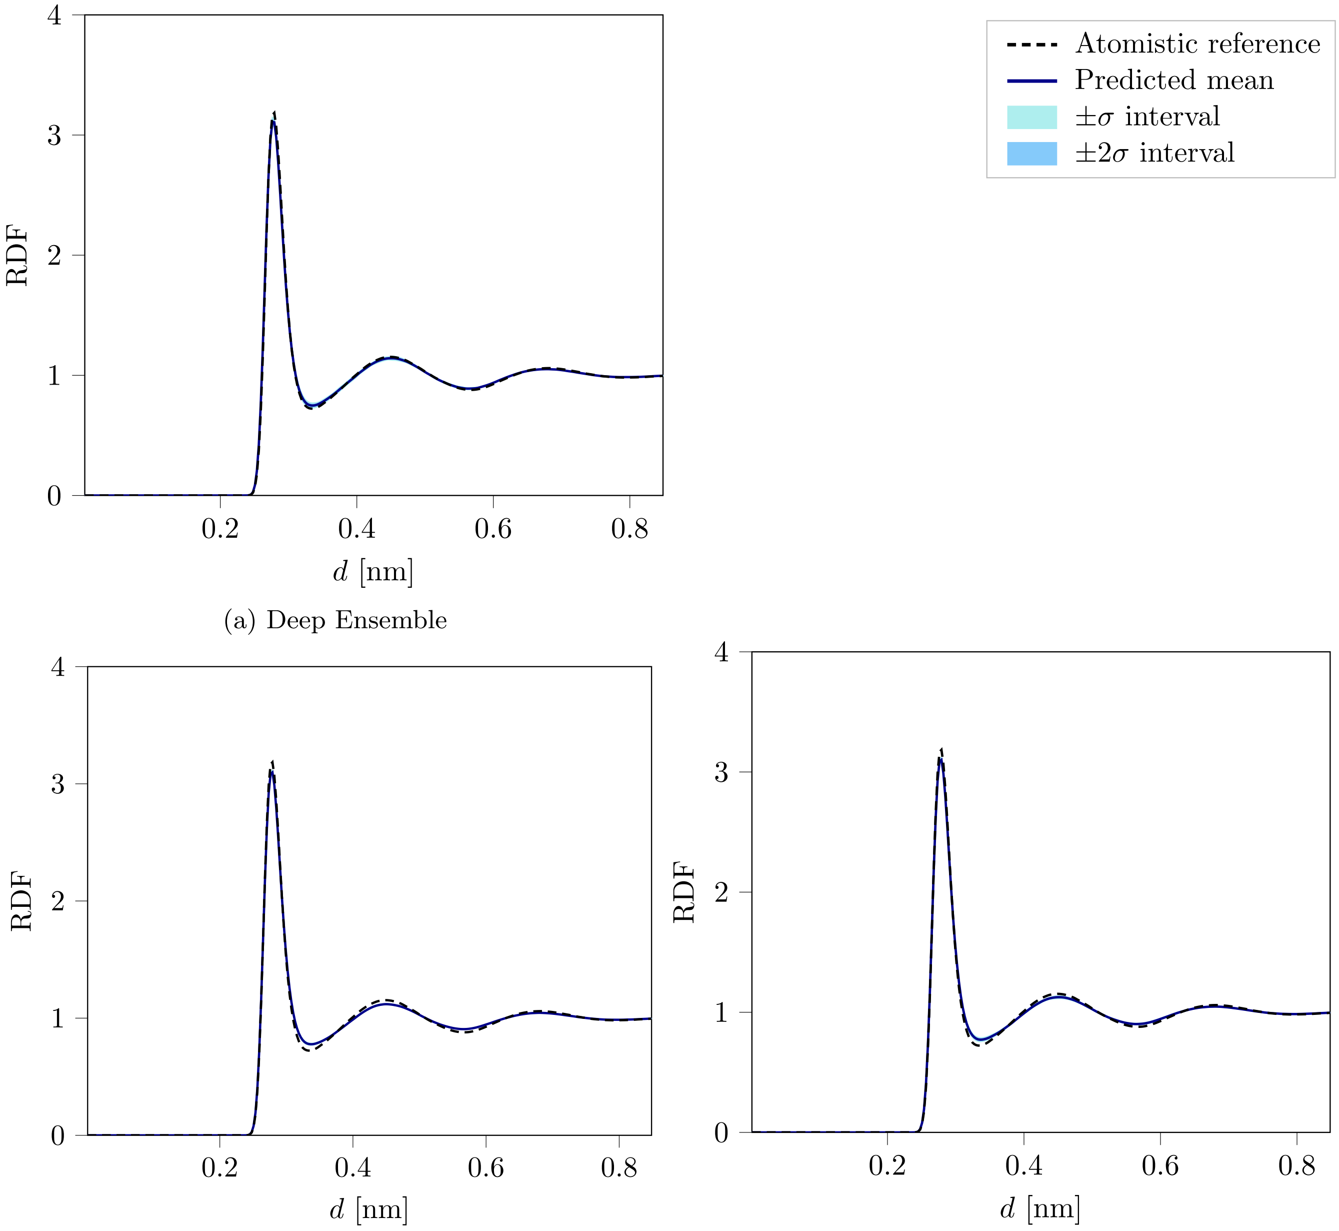


(a) Deep Ensemble

(b) S-pSGLD

(c) M-pSGLD

Figure 4: Radial distribution functions (RDF) at $T = T_{\text{ref}}$. Resulting mean RDF with $\pm\sigma$ and $\pm 2\sigma$ intervals as predicted by the Deep Ensemble ($a$), the single chain pSGLD ($b$) and the multi-chain pSGLD ($c$) schemes at a temperature $T = T_{\text{ref}}$, compared to the atomistic reference.

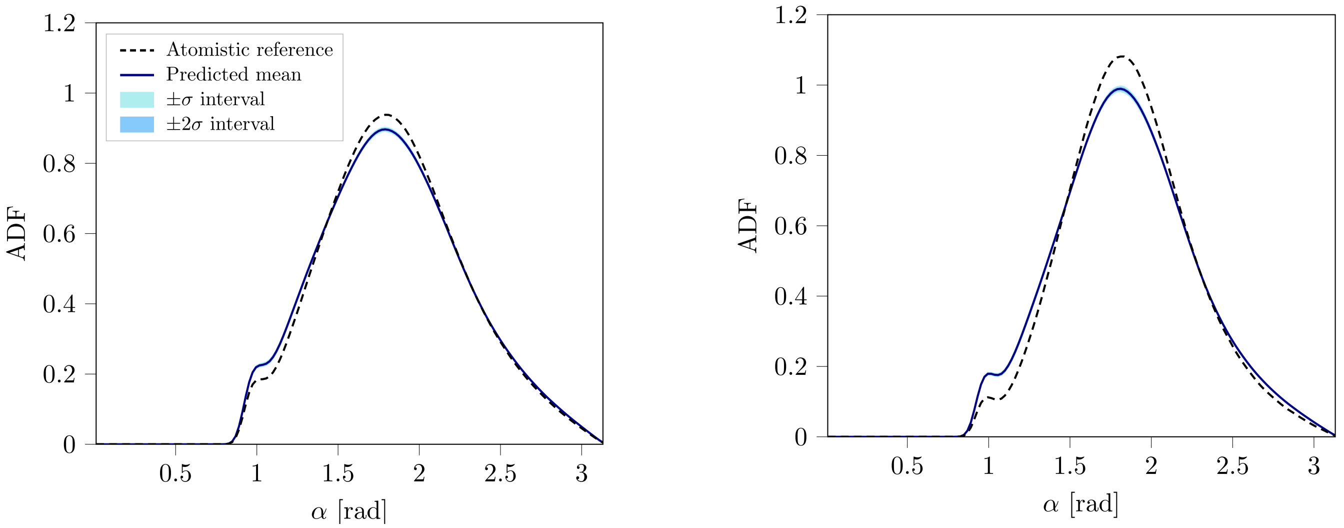


(a) $T = T_{\text{ref}}$ (b) $T = 260\text{K}$

Figure 5: Angular distribution functions (ADF) with uniform weight prior for S-pSGLD. Resulting mean ADF with $\pm\sigma$ and $\pm 2\sigma$ intervals as predicted by the S-pSGLD method with uniform prior over weights and biases at a temperature $T = T_{\text{ref}}$ $(a)$ and $T = 260$ K $(b)$, compared to the atomistic reference.

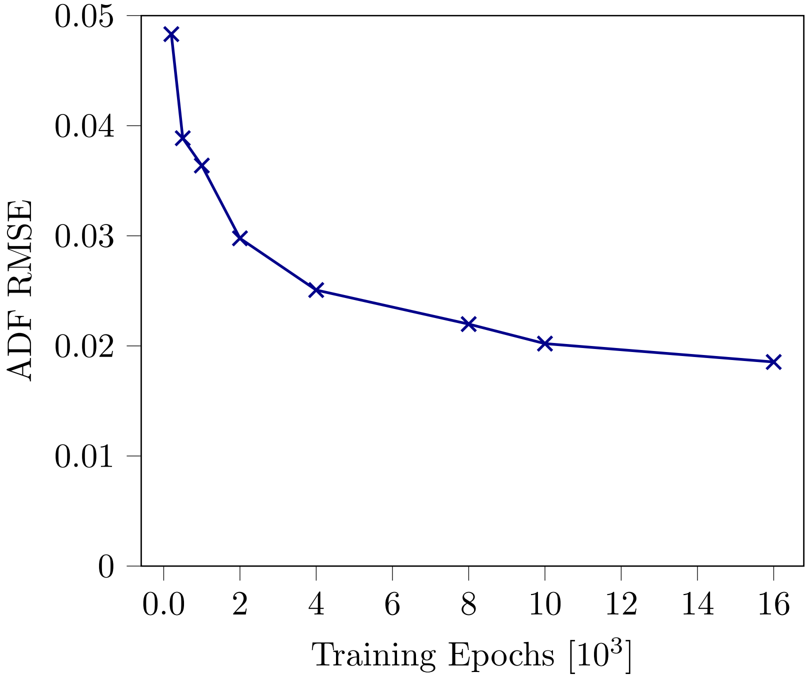


Figure 6: pSGLD chain length variation. Root mean squared error (RMSE) of the mean predicted angular distribution function (ADF) of models sampled by the pSGLD scheme with a single chain of different total lengths. The models are randomly retained after a burn-in period, which is 1000 epochs shorter than the total chain length. Exceptions are chains with lengths of 200, 500 and 1000 epochs, which feature a burn-in period of 200, 400 and 500 epochs, respectively.

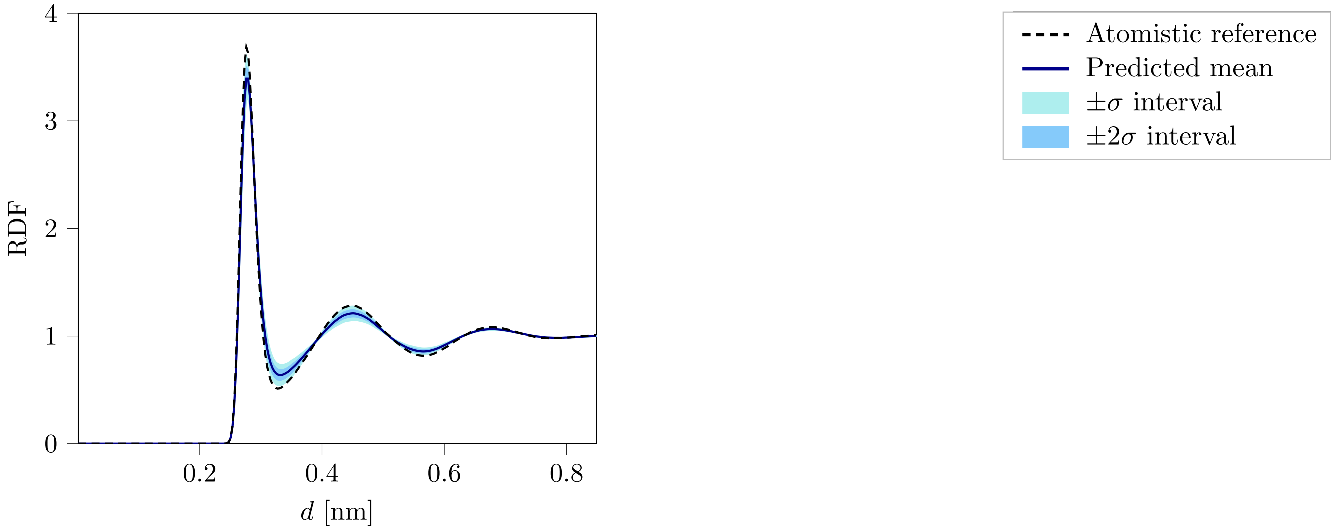


(a) Deep Ensemble

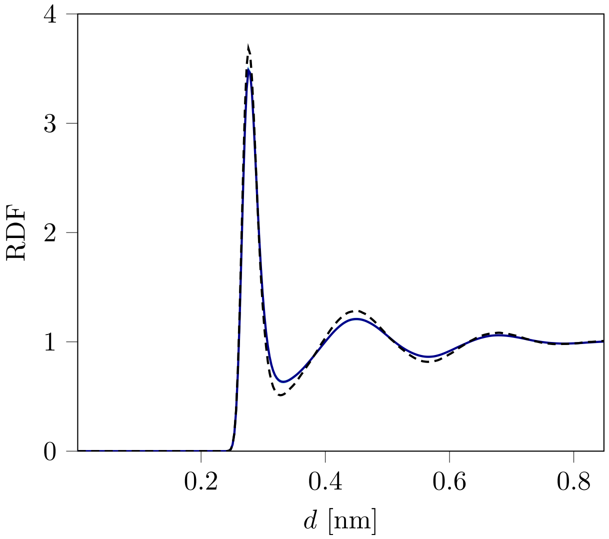


(b) S-pSGLD

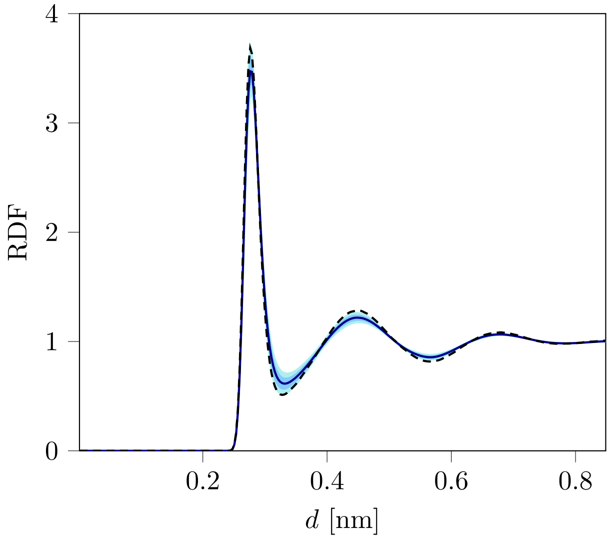


(c) M-pSGLD

Figure 7: Radial distribution functions (RDF) at $T = 260$ K. Resulting mean RDF with $\pm\sigma$ and $\pm 2\sigma$ intervals as predicted by the Deep Ensemble ($a$), the single chain pSGLD ($b$) and the multi-chain pSGLD ($c$) schemes at a temperature $T = 260$ K, compared to the atomistic reference.

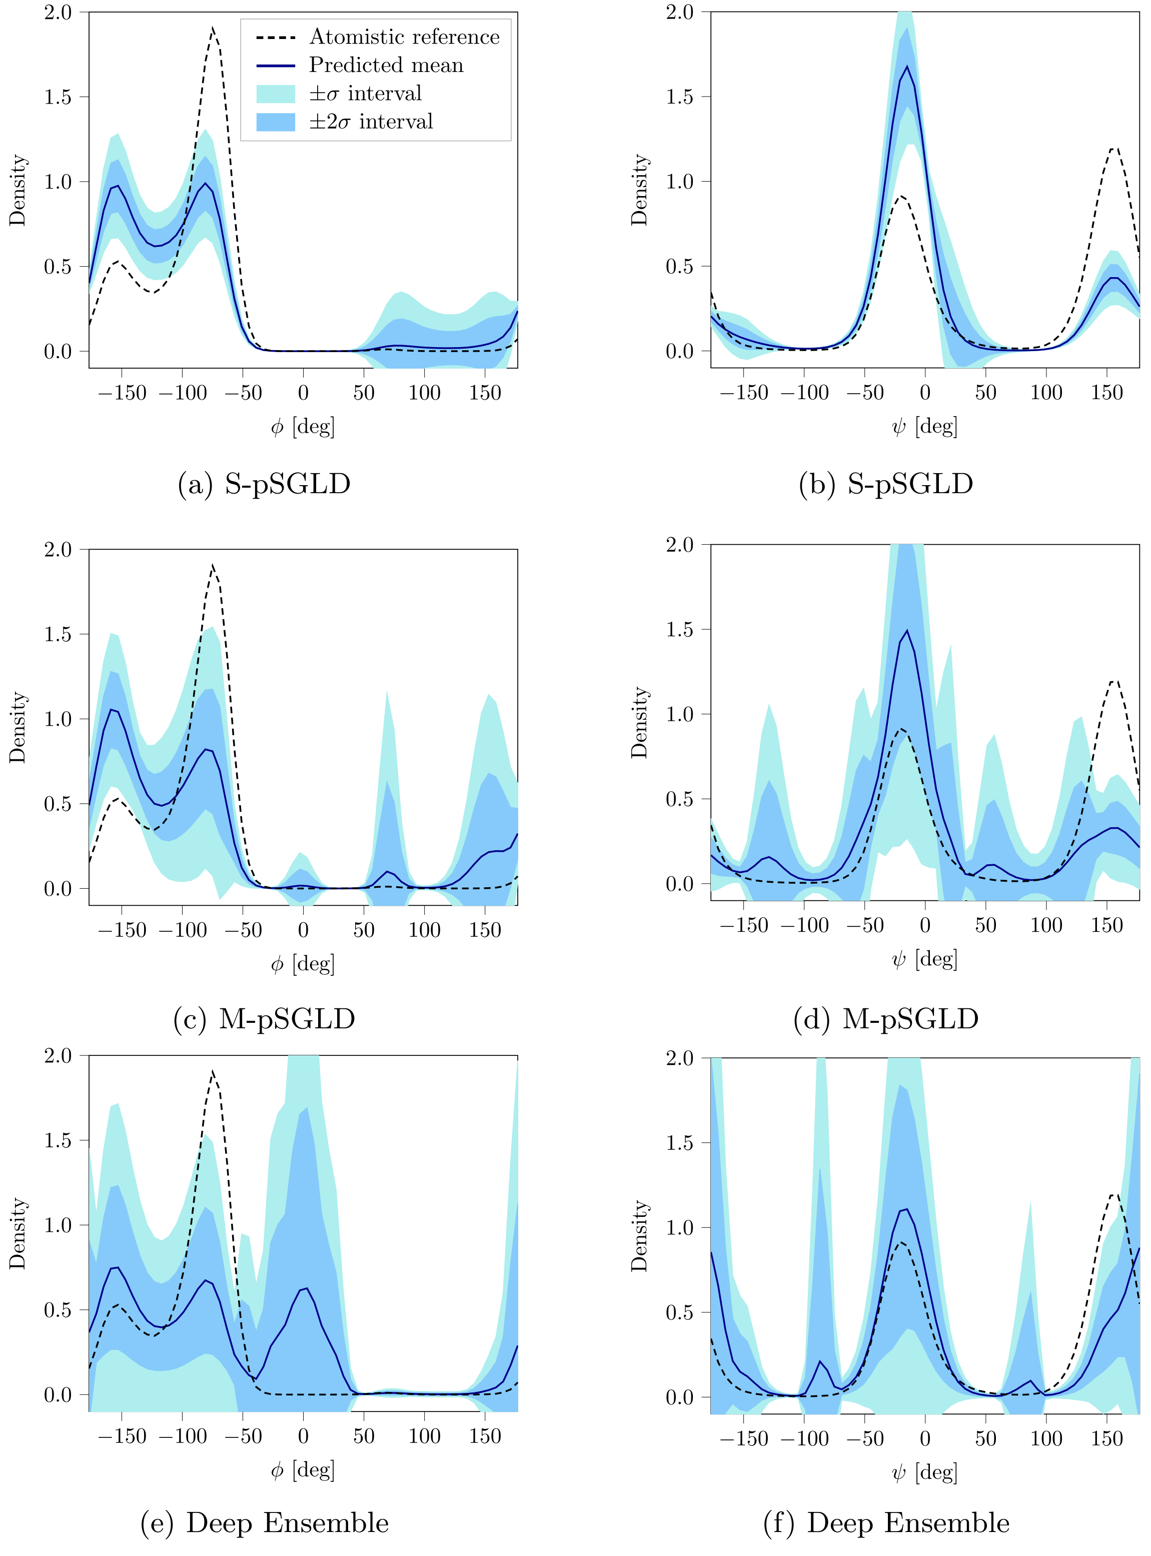


(a) S-pSGLD (b) S-pSGLD

(c) M-pSGLD (d) M-pSGLD

(e) Deep Ensemble (f) Deep Ensemble

Figure 8: Dihedral angle density histograms including potential energy holes. Resulting mean distribution of dihedral angles $\phi$ (left column) and $\psi$ (right column) with $\pm\sigma$ and $\pm 2\sigma$ intervals as predicted by the single chain pSGLD ($a$, $b$), the multi-chain pSGLD ($c$, $d$) and the Deep Ensemble ($e$, $f$) methods based on the 100 ns reference data set, compared to the atomistic reference. No trajectories were removed, except when a potential energy hole resulted in a divergent trajectory. The number of diverged trajectories are 0, 6 and 7 for single chain pSGLD, multi-chain pSGLD, and the Deep Ensemble method, respectively.

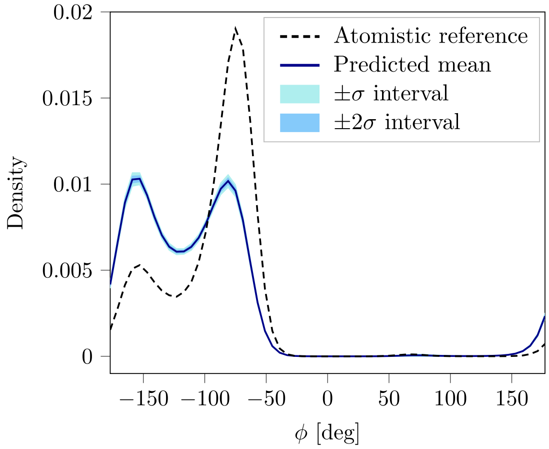


(a) S-pSGLD

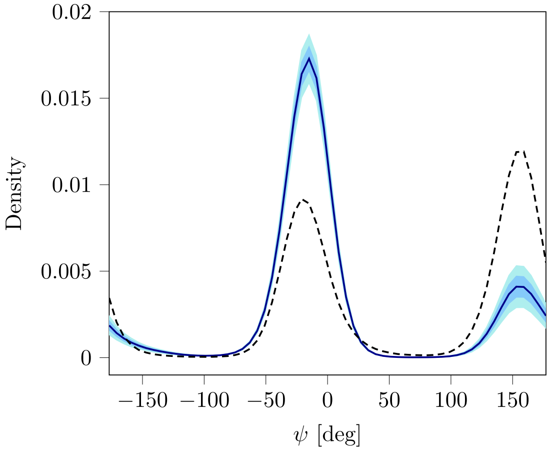


(b) S-pSGLD

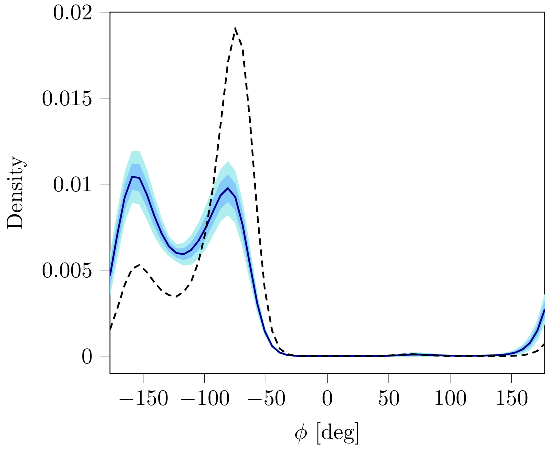


(c) M-pSGLD

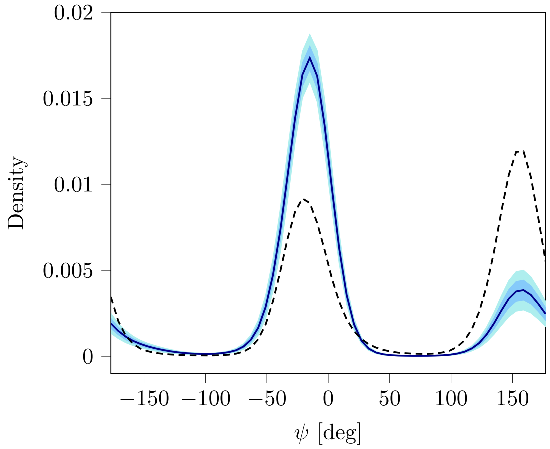


(d) M-pSGLD

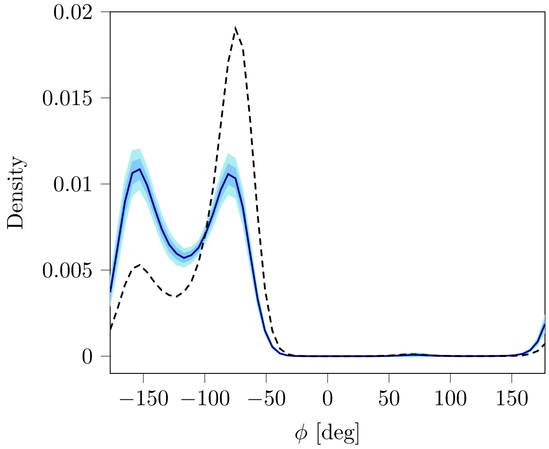


(e) Deep Ensemble

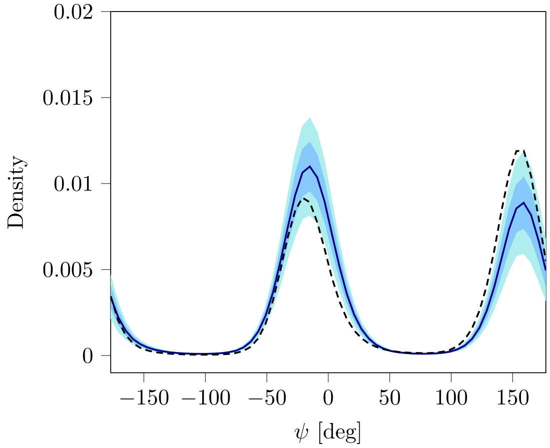


(f) Deep Ensemble

Figure 9: Resulting dihedral angle density histograms from $1\mu s$ training data set. Resulting mean distribution of dihedral angles $\phi$ (left column) and $\psi$ (right column) with $\pm\sigma$ and $\pm 2\sigma$ intervals as predicted by the single chain pSGLD ($a$, $b$), the multi-chain pSGLD ($c$, $d$) and the Deep Ensemble ($e$, $f$) methods, compared to the atomistic reference. Analogous to the results in the main text, we removed 2, 10 and 28 trajectories due to potential energy holes from S-pSGLD, M-pSGLD and the Deep Ensemble method, respectively.

## Supplementary References


[1] Wang, J. *et al.* Machine Learning of Coarse-Grained Molecular Dynamics Force Fields. *ACS Cent. Sci.* **5**, 755–767 (2019).

[2] Husic, B. E. *et al.* Coarse graining molecular dynamics with graph neural networks. *J. Chem. Phys.* **153**, 194101 (2020).

[3] Fu, X. *et al.* Forces are not enough: Benchmark and critical evaluation for machine learning force fields with molecular simulations. In *AI for Science: Progress and Promises Workshop at NeurIPS* (New Orleans, LA, USA, Dec. 2, 2022).

[4] Marrink, S. J., Risselada, H. J., Yefimov, S., Tieleman, D. P. & De Vries, A. H. The MARTINI force field: Coarse grained model for biomolecular simulations. *J. Phys. Chem. B* **111**, 7812–7824 (2007).

[5] Ingólfsson, H. I. *et al.* The power of coarse graining in biomolecular simulations. *Wiley Interdiscip. Rev. Comput. Mol. Sci.* **4**, 225–248 (2014).

[6] Ramakrishnan, R., Dral, P. O., Rupp, M. & Von Lilienfeld, O. A. Big data meets quantum chemistry approximations: The $\Delta$-machine learning approach. *J. Chem. Theory Comput.* **11**, 2087–2096 (2015).

[7] Thaler, S., Stupp, M. & Zavadlav, J. Deep coarse-grained potentials via relative entropy minimization. *J. Chem. Phys.* **157**, 244103 (2022).

[8] Klicpera, J., Groß, J. & Günnemann, S. Directional Message Passing for Molecular Graphs. In *8th International Conference on Learning Representations* (Online, Apr. 26 – May 1, 2020).

[9] Klicpera, J., Giri, S., Margraf, J. T. & Günnemann, S. Fast and uncertainty-aware directional message passing for non-equilibrium molecules. In *Machine Learning for Molecules Workshop at NeurIPS* (Online, Dec. 12, 2020).

[10] Thaler, S. & Zavadlav, J. Learning neural network potentials from experimental data via differentiable trajectory reweighting. *Nat. Commun.* **12**, 6884 (2021).

[11] Hoffman, M. D. & Gelman, A. The no-u-turn sampler: adaptively setting path lengths in hamiltonian monte carlo. *J. Mach. Learn. Res.* **15**, 1593–1623 (2014).

[12] Hansen, L. & Salamon, P. Neural network ensembles. *IEEE Trans. Pattern Anal. Machine Intell.* **12**, 993–1001 (1990).

[13] Lakshminarayanan, B., Pritzel, A. & Blundell, C. Simple and scalable predictive uncertainty estimation using deep ensembles. In Guyon, I. *et al.* (eds.) *Advances in Neural Information Processing Systems*, vol. 30 (Curran Associates, Inc., Long Beach, CA, USA, Dec. 4–9, 2017).

[14] Welling, M. & Teh, Y. W. Bayesian learning via stochastic gradient langevin dynamics. In *Proceedings of the 28th International Conference on Machine Learning*, 681–688 (Omnipress, 2600 Anderson St, Madison, WI, USA, Bellevue, WA, USA, Jun. 28 – Jul. 2, 2011).

[15] Thompson, A. P., Plimpton, S. J. & Mattson, W. General formulation of pressure and stress tensor for arbitrary many-body interaction potentials under periodic boundary conditions. *J. Chem. Phys.* **131**, 154107 (2009).

[16] Das, A. & Andersen, H. C. The multiscale coarse-graining method. iii. a test of pairwise additivity of the coarse-grained potential and of new basis functions for the variational calculation. *J. Chem. Phys.* **131**, 034102 (2009).

[17] Dunn, N. J. & Noid, W. Bottom-up coarse-grained models that accurately describe the structure, pressure, and compressibility of molecular liquids. *J. Chem. Phys.* **143**, 243148 (2015).
